# Supplementary material for: Explaining Predictions from Machine Learning Models: Algorithms, Users, and Pedagogy
Source: arXiv:2209.05084 source file (2022-09-12)
Supplement: Supplementary file 1 [file appendix.tex]

%!TEX root = ../main.tex

\section*{Appendix}
\label{section:hyperparameters}
Here we detail the FOCUS hyperparameters across the \numprint{42} settings in Experiments 1 and 2. $\sigma$ indicates the steepness of the sigmoid function in Equation~\ref{eq:sigma}; $\tau$ is the temperature of the softmax in Equation~\ref{eq:tau}; $\beta$ is the trade-off parameter in Equation~\ref{eq:approxloss}; $\alpha$ is the learning rate of Adam. 

%EUCLIDEAN
\begin{table}[h]
\centering
\caption{FOCUS hyperparameters used in Experiment 1 comparing FOCUS with FT using Euclidean distance.}
\label{table:hyperparameters-euc}
\begin{tabular}{lcccrrrr}
\toprule
\textbf{Dataset}                   & \textbf{Model}       & \textbf{Num Trees}   & \textbf{Max Depth}   & $\sigma$ & $\tau$ & $\beta$ & $\alpha$ \\ \midrule
%\textbf{Dataset}                   & \textbf{Model}       & \textbf{Num}   & \textbf{Max}   & $\sigma$ & $\tau$ & $\beta$ & $\alpha$ \\
%			                   & 			       & \textbf{Trees}   & \textbf{Depth}   &  &  &  &  \\ \midrule
	                 & DT                   & 1                                  & 2                                  & 1  & 10 & 0.05 & 0.001    	 \\
\textsc{Wine}                   & RF                   & 500                                & 4                                  & 10 & 2  & 0.05 & 0.005      	 \\
\textsc{}                          & AB                   & 100                                & 4                                  & 5  & 1  & 0.05 & 0.005      	 \\ \midrule
\multirow{3}{*}{\textsc{HELOC}}    & DT                   & 1                                  & 4                                  & 2  & 10 & 0.05 & 0.001	    \\
                                   & RF                   & 500                                & 4                                  & 10 & 5  & 0.05 & 0.005      	\\
                                   & AB                   & 100                                & 8                                  & 10 & 1  & 0.05 & 0.001  	   \\ \midrule
\multirow{3}{*}{\textsc{COMPAS}}   & DT                   & 1                                  & 4                                  & 6  & 10 & 0.05 & 0.005       \\
                                   & RF                   & 500                                & 4                                  & 7  & 3  & 0.01 & 0.001      \\
                                   & AB                   & 100                                & 2                                  & 10 & 1  & 0.01 & 0.005	\\ \midrule
\multirow{3}{*}{\textsc{Shopping}} & DT                   & 1                                  & 4                                  & 2  & 10 & 0.05 & 0.005     \\
                                   & RF                   & 500                                & 8                                  & 5  & 5  & 0.05 & 0.005      \\
                                   & AB                   & 100                                & 2                                 & 10 & 1  & 0.05 & 0.001      \\ \bottomrule
\end{tabular}
\end{table}

\vspace{-5em}

%COSINE
\begin{table}[h]
\centering
\caption{FOCUS hyperparameters used in Experiment 1 comparing FOCUS with FT using Cosine distance.}
\label{table:hyperparameters-cos}
\begin{tabular}{lcccrrrr}
\toprule
\textbf{Dataset}                   & \textbf{Model}       & \textbf{Num Trees}   & \textbf{Max Depth}   & $\sigma$ & $\tau$ & $\beta$ & $\alpha$ \\ \midrule
	                  & DT                   & 1                                  & 2                                  & 1  & 10 & 0.05 & 0.005      	 \\
\textsc{Wine}                   & RF                   & 500                                & 4                                  & 10 & 1  & 0.05 & 0.005      	 \\
                        & AB                   & 100                                & 4                                  & 1  & 1  & 0.01 & 0.005      	 \\ \midrule
\multirow{3}{*}{\textsc{HELOC}}    & DT                   & 1                                  & 4                                  & 2  & 10 & 0.05 & 0.005  	    \\
                                   & RF                   & 500                                & 4                                  & 5  & 5  & 0.05 & 0.005       	\\
                                   & AB                   & 100                                & 8                                  & 1  & 1  & 0.05 & 0.005   	   \\ \midrule
\multirow{3}{*}{\textsc{COMPAS}}   & DT                   & 1                                  & 4                                  & 10 & 10 & 0.05 & 0.005       \\
                                   & RF                   & 500                                & 4                                  & 10 & 6  & 0.01 & 0.005       \\
                                   & AB                   & 100                                & 2                                  & 10 & 1  & 0.05 & 0.005       	\\ \midrule
\multirow{3}{*}{\textsc{Shopping}} & DT                   & 1                                  & 4                                  & 10 & 10 & 0.05 & 0.001      \\
                                   & RF                   & 500                                & 8                                  & 1  & 1  & 0.01 & 0.001       \\
                                   & AB                   & 100                                & 2                                  & 10 & 5  & 0.05 & 0.001      \\ \bottomrule
\end{tabular}
\end{table}

%MANHATTAN

\begin{table}[h]
\centering
\caption{FOCUS hyperparameters used in Experiment 1 comparing FOCUS with FT using Manhattan distance.}
\label{table:hyperparameters-manhat}
\begin{tabular}{lcccrrrr}
\toprule
\textbf{Dataset}                   & \textbf{Model}       & \textbf{Num Trees}   & \textbf{Max Depth}   & $\sigma$ & $\tau$ & $\beta$ & $\alpha$ \\ \midrule
                    & DT                   & 1                                  & 2                                  & 1  & 10 & 0.05 & 0.001     	 \\
\textsc{Wine}                   & RF                   & 500                                & 4                                  & 10 & 10 & 0.01 & 0.005    	 \\
\textsc{}                          & AB                   & 100                                & 4                                  & 6  & 1  & 0.01 & 0.005     	 \\ \midrule
\multirow{3}{*}{\textsc{HELOC}}    & DT                   & 1                                  & 4                                 & 2  & 10 & 0.05 & 0.001  	    \\
                                   & RF                   & 500                                & 4                                 & 5  & 5  & 0.01 & 0.005     	\\
                                   & AB                   & 100                                & 8                                  & 4  & 1  & 0.05 & 0.001  	   \\ \midrule
\multirow{3}{*}{\textsc{COMPAS}}   & DT                   & 1                                  & 4                                  & 6  & 10 & 0.01 & 0.005      \\
                                   & RF                   & 500                                & 4                                   & 4  & 1  & 0.05 & 0.001       \\
                                   & AB                   & 100                                & 2                                  & 5  & 10 & 0.05 & 0.005  	\\ \midrule
\multirow{3}{*}{\textsc{Shopping}} & DT                   & 1                                  & 4                                  & 2  & 10 & 0.05 & 0.005    \\
                                   & RF                   & 500                                & 8                                  & 10 & 1  & 0.05 & 0.001       \\
                                   & AB                   & 100                                & 2                                  & 10 & 1  & 0.05 & 0.001     \\ \bottomrule
\end{tabular}
\end{table}

%MAHALANOBIS
\makeatletter
\setlength{\@fptop}{0pt}
\makeatother

\begin{table}[ht!]
\centering
\caption{FOCUS hyperparameters used in Experiment 2 comparing FOCUS with DACE using Mahalanobis distance.}
\label{table:hyperparameters-mahal}
\begin{tabular}{lcccrrrr}
\toprule
\textbf{Dataset}                   & \textbf{Model}       & \textbf{Num Trees}   & \textbf{Max Depth}   & $\sigma$ & $\tau$ & $\beta$ & $\alpha$ \\ \midrule
\textsc{Wine}                      & DT                   & 1                                  & 2                                  & 5  & 10 & 0.01  & 0.001       	 \\ \midrule
\textsc{HELOC}   & DT                   & 1                                  & 4                                  & 5  & 10 & 0.01  & 0.001   	    \\ \midrule

\multirow{2}{*}{\textsc{COMPAS}}   & DT                   & 1                                  & 4                                  & 5  & 10 & 0.01  & 0.005   \\
                                   & AB                   & 100                                & 2                                  & 4  & 2  & 0.005 & 0.001      	\\ \midrule
\multirow{2}{*}{\textsc{Shopping}} & DT                   & 1                                  & 4                                 & 4  & 10 & 0.01  & 0.005 \\
                                   & AB                   & 100                                & 2                                  & 10 & 1  & 0.01  & 0.001      \\ \bottomrule
\end{tabular}
\end{table}
