# Supplementary material for: Explaining Predictions from Machine Learning Models: Algorithms, Users, and Pedagogy
Source: arXiv:2209.05084 source file (2022-09-12)
Supplement: Supplementary file 2 [file appendix_final.tex]

\section{Results Table Including Standard Deviations}
Here we show Table 2 from the manuscript including standard deviations. 
We report standard deviation for two metrics: \textit{Explanation Size} and \textit{Sparsity}, since both of these involve taking the mean over the entire dataset. 
Standard deviation does not apply to \textit{Fidelity} or \textit{Accuracy} because these metrics represent a proportion as opposed to a mean.

\begin{table}[h]
\centering
\caption*{Table 2: Results comparing our method (denoted \OurShort{}) to \baserand{}, \basekeep{}, and \baserm{}. Below each metric, $\blacktriangledown$ indicates a low value is desirable, while $\blacktriangle$ indicates a high value is desirable.}
\label{table:results}
%\setlength{\tabcolsep}{4pt}
%\footnotesize{
\resizebox{\textwidth}{!}{\begin{tabular}{lrrrrrrrrrrrr}
\toprule
\multicolumn{1}{c}{} & \multicolumn{4}{c}{\synfour{}}                                                                                                                 & \multicolumn{4}{c}{\synfive{}}                                                                                                                   & \multicolumn{4}{c}{\synone{}}                                                                                                                  \\ 
\cmidrule(r){2-5}\cmidrule(r){6-9}\cmidrule{10-13} 
               & \multicolumn{1}{c}{\textit{Fid.}} & \multicolumn{1}{c}{\textit{Size}} & \multicolumn{1}{c}{\textit{Spars.}} & \multicolumn{1}{c}{\textit{Acc.}} & \multicolumn{1}{c}{\textit{Fid.}} & \multicolumn{1}{c}{\textit{Size}} & \multicolumn{1}{c}{\textit{Spars.}} & \multicolumn{1}{c}{\textit{Acc.}} & \multicolumn{1}{c}{\textit{Fid.}} & \multicolumn{1}{c}{\textit{Size}} & \multicolumn{1}{c}{\textit{Spars.}} & \multicolumn{1}{c}{\textit{Acc.}} \\

% & \multicolumn{1}{c}{$\downarrow$} &\multicolumn{1}{c}{$\downarrow$} &\multicolumn{1}{c}{$\uparrow$} & \multicolumn{1}{c}{$\uparrow$} & \multicolumn{1}{c}{$\downarrow$} &\multicolumn{1}{c}{$\downarrow$} &\multicolumn{1}{c}{$\uparrow$} & \multicolumn{1}{c}{$\uparrow$} & \multicolumn{1}{c}{$\downarrow$} &\multicolumn{1}{c}{$\downarrow$} &\multicolumn{1}{c}{$\uparrow$} & \multicolumn{1}{c}{$\uparrow$} \\

Method & \multicolumn{1}{c}{$\blacktriangledown$} &\multicolumn{1}{c}{$\blacktriangledown$} &\multicolumn{1}{c}{$\blacktriangle$} & \multicolumn{1}{c}{$\blacktriangle$} & \multicolumn{1}{c}{$\blacktriangledown$} &\multicolumn{1}{c}{$\blacktriangledown$} &\multicolumn{1}{c}{$\blacktriangle$} & \multicolumn{1}{c}{$\blacktriangle$} & \multicolumn{1}{c}{$\blacktriangledown$} &\multicolumn{1}{c}{$\blacktriangledown$} &\multicolumn{1}{c}{$\blacktriangle$} & \multicolumn{1}{c}{$\blacktriangle$} \\
\midrule
\baserand{}               & \textbf{0.00}                     & 4.70   $\pm$       4.28                    & 0.79     $\pm$ 0.07                           & 0.63                               & \textbf{0.00}                     & 9.06    $\pm$ 6.81                          & 0.75      $\pm$ 0.07                          & 0.77                               & \textbf{0.00}                     & 503.31   $\pm$ 332.61                         & 0.58   $\pm$ 0.10                             & 0.17                              \\
\basekeep{}                 & 0.32                              & 15.64      $\pm$ 12.36                       & 0.13       $\pm$ 0.06                         & 0.45                               & 0.32                              & 29.30      $\pm$16.53                       & 0.09      $\pm$ 0.04                          & 0.72                               & 0.60                              & 504.18    $\pm$ 567.92                        & 0.05      $\pm$ 0.05                          & 0.18                              \\
\baserm{}              & 0.46                              & 2.11          $\pm$ 1.04                    & 0.89         $\pm$ 0.04                       & ---                                  & 0.61                              & 2.27         $\pm$ 1.28                     & 0.92      $\pm$ 0.04                          & ---                                  & 0.21                              & 10.56      $\pm$ 20.11                       & 0.97     $\pm$ 0.04                           & \textbf{0.99}                     \\

% \gnnexpshort{} ($S=$ GT) &  0.55 &	6.00 & 0.57 &	0.46 &	0.35 &	11.83 &	0.53 &	0.74 &	0.82 &	6.00 &	0.79 &	0.24    \\

\midrule
\OurShort{}               & 0.21                              & \textbf{2.09}     $\pm$ 2.21                & \textbf{0.90}    $\pm$ 0.07                   & \textbf{0.94}                      & 0.07                              & \textbf{1.47}    $\pm$0.77                 & \textbf{0.94}    $\pm$ 0.04                   & \textbf{0.96}                      & 0.39                              & \textbf{2.39}    $\pm$ 1.39                 & \textbf{0.99}      $\pm$ 0.01                 & 0.96                 \\
\bottomrule
\end{tabular}}
%}
\end{table}

All differences between \OurMethod{} and the baselines are statistically significant with $\alpha=0.01$ using a $t$-test, with two exceptions: \OurMethod{} vs. \baserm{} on the \synfive{} dataset, for (i) \textit{Explanation Size} and (ii) \textit{Sparsity}. However, \OurMethod{} outperforms \baserm{} significantly on \textit{Fidelity} and \textit{Accuracy} ($\alpha=0.01$).

We do not calculate standard deviations for Table 3, where we compare against \gnnexplainer{}, since we cannot evaluate \gnnexplainer{} on \textit{Explanation Size} or \textit{Sparsity}. This is because the user must specify the \textit{Explanation Size} in advance (see Sections 6.2, 7.2). We can only evaluate \gnnexplainer{} on \textit{Fidelity} and \textit{Accuracy}, neither of which require standard deviation calculations since they represent proportions.
